# Supplementary material for: DynOMo: Online Point Tracking by Dynamic Online Monocular Gaussian Reconstruction
Source: arXiv:2409.02104 source file (2025-03-12)
Supplement: Supplementary file 1 [file supp_jono.tex]

\begin{table*}[!thp]
    \centering
    \footnotesize
    \setlength{\tabcolsep}{4.2pt}
    %\resizebox{0.95\linewidth}{!}{
    \begin{tabular}{l|ccc|ccc|ccc}
    \toprule
        %& \multicolumn{6}{c}{\textit{3DIoU}}\\
        Method & $MTE_{2D}$ $\downarrow$ & $S_{2D}$ $\uparrow$ & $\delta_{avg, 2D}$ $\uparrow$ & \%1 & \%8 & \%16 & PSNR $\uparrow$ & SSIM $\uparrow$  & LPIPS $\downarrow$ \\
        \midrule
        \midrule
        D-3DGS \cite{luiten2023dynamic} & 10.5 & 76.8 & 57.4 & 20.6 & 75.9 & 82.5 & 33.2 & 0.96 & 0.05 \\
        D-3DGS-M & 23.3 & 41.0 & 30.6& 14.8 & 37.9 & 47.5  & \textbf{39.6}  & \textbf{0.98} & \textbf{0.03} \\
        D-3DGS-M$_f$ & 29.5 & 43.5 & 28.3 & 9.7 & 38.7 & 46.3  & 37.8 & 0.97 & 0.06 \\
        \midrule
        \method-DA \cite{Yang2024depthanything} & \textbf{3.7} & 83.7 & 59.0 & 19.6 & 80.3 & 88.7 & 32.5 & 0.96 & 0.90 \\
        % \method (D-3DGS-D) & 9.3 & 73.8 & 52.7 & 31.6 & 0.96 & 0.10 & & \\
        \method-D-3DGS-D & 6.3 & \textbf{85.7} & \textbf{61.8} & \textbf{25.3} & \textbf{83.6} & \textbf{90.3} & 31.9 & 0.96 & 0.09 \\
        \method-S-D-3DGS-D  \textcolor{red}{incomplete} & 8.1 &  73.1 & 47.0 & 1.0 & 69.0 & 82.3 & 27.1 & 0.89 & 0.21 \\
        % \method (DepthAnything) & 7.6 & 68.4 & 53.4  & 19.2 & 69.5 & 67.3  & 32.1 & 0.96 & 0.11\\
        % \method-D-3DGS-PC & 26.7 & 54.6 & 36.4  & 11.3 & 51.3 & 59.8 & 37.6 & 0.99 & 0.05 \\
    \bottomrule
    \end{tabular}
    \caption{\textbf{Comparison on Panoptic Studio \cite{luiten2023dynamic} for 2D Point Tracking:} We compare our performance on the updated setting explained in \cref{subsec:dataset}. D-3DGS-M is \cite{luiten2023dynamic} optimized using a single camera. In D-3DGS-M$_f$ we reduce the number of iterations during optimization. We observe that despite our approach only has access to one single view, our 2D point tracking outperforms the one obtained by \cite{luiten2023dynamic}. Note that since we optimize for point tracking rather than novel-view synthesis, we report rendering metrics on training views. Hence, that this is just for reference not for SOTA comparisons.}
    %}
    \label{tab:jono2d}
\end{table*}

\begin{table}[t]
    \centering
    \footnotesize
    \setlength{\tabcolsep}{4.2pt}
    %\resizebox{0.95\linewidth}{!}{
    \begin{tabular}{l|ccc}
    \toprule
        %& \multicolumn{6}{c}{\textit{3DIoU}}\\
        Method & $MTE_{3D}$ $\downarrow$ & $S_{3D}$ $\uparrow$ & $\delta_{avg, 3D}$ $\uparrow$ \\
        \midrule
        \midrule
        D-3DGS \cite{luiten2023dynamic} & 13.7 & 86.8 & 43.7 \\
        D-3DGS-M & 56.0 & 44.5 & 7.3  \\
        D-3DGS-M$_f$ & 50.5 & 43.9 & 6.6  \\
        \midrule
         \method-DA \cite{Yang2024depthanything} & 70.7 & 25.4 & 0.7 \\  % not_higher_lr_original_size_transformed from 3D
        % \method-D-3DGS-PC & 31.1 & 71.2 & 11.7  \\ % not_higher_lr_normal_size_jono_pc_orig_size from 3D
        \method-D-3DGS-D & 26.1 & 73.0 & 12.7  \\ % not_higher_lr_orig_size_transformed_jono_depth from 3D
        % \method (DepthAnything) & 147.7 & 0.0 & 0.3  \\ % not_higher_lr_original_size_transformed
       \method-S-D-3DGS-D \textcolor{red}{incomplete} & 31.6 & 62.0 & 10.0 \\
    \bottomrule
    \end{tabular}
    \caption{\textbf{Comparison on Panoptic Studio \cite{luiten2023dynamic} for 3D Point Tracking:} We compare our performance to on 3D trajectories. D-3DGS-M is \cite{luiten2023dynamic} optimized using a single camera. In D-3DGS-M$_f$ we reduce the number of iterations during optimization. We observe that $MTE_{3D}$ and $\delta_{avg, 3D}$ are considerably lower than D-3DGS. However, our performance significantly ourperforms the monocular setup of \cite{luiten2023dynamic} D-3DGS-M. This shows that our optimization indeed enforces Gaussiam particles to move appropirately in the 3D space.}
    %}
    \label{tab:jono3d}
\end{table}
